# Supplementary material for: Simulations of Bosonic BMN Matrix Model
Source: arXiv:2007.04920 source file (2020-06-17)
Supplement: Supplementary file 1 [file appendix.tex]

\chapter{A1}
